# Supplementary material for: Active Token Mixer
Source: arXiv:2203.06108 source file (2022-12-23)
Supplement: Supplementary file 1 [file supp_ablation_atm.tex]

\begingroup

\setlength{\tabcolsep}{3pt}
\begin{NiceTabular}{@{}lcclcl@{}}[code-before=
\rectanglecolor{\rc}{4-2}{4-6}
\rectanglecolor{\rc}{6-2}{6-6}
\rectanglecolor{\rc}{8-2}{8-6}
]

\hline
& & \multicolumn{2}{c}{Semantic FPN} & \multicolumn{2}{c}{Mask R-CNN} \\
Backbone & Neck & FLOPS & mIoU & FLOPS & AP$^b$ \\
\hline

\multirow{2}{*}{\ourst}
& FPN         & 42.4 & 45.8
            & 251.1 & 44.8 \\
& ATMFPN  
    & 41.4 & 46.5\tcg{\large$_{\uparrow0.7}$}
    & 247.0 & 45.6\tcg{\large$_{\uparrow0.8}$}   \\
\hline
\end{NiceTabular}
\endgroup
