# Supplementary material for: Active Token Mixer
Source: arXiv:2203.06108 source file (2022-12-23)
Supplement: Supplementary file 2 [file supp_ablation.tex]

% \resizebox{0.5\textwidth}{!}{    
\begin{NiceTabular}{c|c|ccc|c|c}[
code-before=
\rectanglecolor{\rc}{3-1}{3-7}
]
\hline
\multirow{2}{*}{ID.}& \multirow{2}{*}{Fusion ways} & \multirow{2}{*}{\#P.(M)\thickspace} & \multirow{2}{*}{FLOPs(G)\thickspace} & \multirow{2}{*}{Top-1 acc.} & \multicolumn{2}{c}{COCO} \\
\cline{6-7}
&&&&&\thickspace AP$^b$\thickspace&\thickspace AP$^m$\thickspace \\
\hline

% =====> 
\ding{172} & Three branches & 26.9 & 3.9 &
    82.0 & 45.6 & 41.5 \\
% \hline
\ding{173} & Identity branch & 26.9 & 3.9 
    & 81.6\color{red!65}{\large$_{\downarrow0.2}$} 
    & 45.1\color{red!65}{\large$_{\downarrow0.5}$}
    & 41.4\color{red!65}{\large$_{\downarrow0.1}$} \\
    
\ding{173} & Parameters & 25.1 & 3.9 
    & 80.3\color{red!65}{\large$_{\downarrow1.5}$} 
    & 44.5\color{red!65}{\large$_{\downarrow1.1}$} 
    & 40.5\color{red!65}{\large$_{\downarrow1.0}$} \\

\hline
\end{NiceTabular}
% 		}

\vspace{-0.5cm}
