# Supplementary material for: Active Token Mixer
Source: arXiv:2203.06108 source file (2022-12-23)
Supplement: Supplementary file 3 [file supp_cascade_mask.tex]

\begingroup

% \resizebox{\textwidth}{!}{    
\begin{NiceTabular}{@{}l|c@{\hspace{5pt}}c|ccc|ccc|ccc|ccc@{}}[code-before=
\rectanglecolor{\rc}{3-1}{3-15}
\rectanglecolor{\rc}{9-1}{9-15}
\rectanglecolor{\rc}{14-1}{14-15}
\rectanglecolor{\rc}{18-1}{18-15}
]
\hline
\multirow{2}{*}{Model}
& \multirow{2}{*}{\makecell{\#P.}} 
& \multirow{2}{*}{\makecell{FLOPs}} 
& \multicolumn{6}{c}{Cascade Mask R-CNN 1$\times$ MS} 
& \multicolumn{6}{c}{Casecade Mask R-CNN 3$\times$ MS} \\
% \cline{4-15}

 & & & AP$^b$ & AP$^b_{50}$ & AP$^b_{75}$ & AP$^m$ & AP$^m_{50}$ & AP$^m_{75}$ & AP$^b$ & AP$^b_{50}$ & AP$^b_{75}$ & AP$^m$ & AP$^m_{50}$ & AP$^m_{75}$ \\
\hline

\oursxt & 73 & 693
    & 47.6 & 66.5 & 51.4 & 41.3 & 63.6 & 44.6
    & 50.0 & 68.7 & 54.4 & 43.5 & 66.2 & 46.8 \\
\hline

ResNet-50 & 82 & 739 
    &- &- &- &- &- &-
    & 46.3 & 64.3 & 50.5 & 40.1 & 61.7 & 43.4 \\ % cswin
Deit-S  & 80 & 889 
    &- &- &- &- &- &-
    & 48.0 & 67.2 & 51.7 & 41.4 & 64.2 & 44.3 \\ %asmlp
Swin-T & 86 & 745
    & 48.1 & 67.1 & 52.2 & 41.7 & 64.4 & 45.0
    & 50.4 & 69.2 & 54.7 & 43.7 & 66.6 & 47.3 \\ % github
% PVTv2-B2-Li \cite{wang2021pvtv2} & 80 & 725
%     &- &- &- &- &- &-
%     & 50.9 & 69.5 & 55.2 & -& -& -\\ % pvtv2
% PVTv2-B2 \cite{wang2021pvtv2} & 83 & 788
%     &- &- &- &- &- &-
%     & 51.1 & 69.8 & 55.3 & -& -& -\\ % pvtv2
AS-MLP-T & 86 & 739
    &- &- &- &- &- &-
    & 50.1 & 68.8 & 54.3 & 43.5 & 66.3 & 46.9 \\ % asmlp
Shift-T & 86 & 743
    &- &- &- &- &- &-
    & 50.3 & 68.6 & 54.7 & 43.4 & 66.2 & 47.0 \\
\ourst & 85 & 730
    & \textbf{49.4} & 68.3 & 53.4 & \textbf{42.8} & 65.7 & 45.9
    & \textbf{51.0} & 69.8 & 55.3 & \textbf{44.4} & 67.4 & 48.3 \\ % done
\hline

X101-32 & 101 & 819 
    &- &- &- &- &- &-
    & 48.1 & 66.5 & 52.4 & 41.6 & 63.9 & 45.2 \\ % cswin
Swin-S & 107 & 838 
    & 50.1 & 69.3 & 54.2 & 43.2 & 66.4 & 46.8 % ours
    & 51.9 & 70.0 & 56.3 & 45.0 & 68.2 & 48.8 \\ % github
ASMLP-S & 107 & 824
    &- &- &- &- &- &-
    & 51.1 & 69.8 & 55.6 & 44.2 & 67.3 & 48.1 \\
Shift-S & 107 & 827
    &- &- &- &- &- &-
    & 50.9 & 69.2 & 55.2 & 44.0 & 67.0 & 47.6 \\
% \ourss & 96 & 790
%     & 51.0 & 70.3 & 55.4 & 44.2 & 67.5 & 47.6
%     & 51.5 & 70.3 & 55.9 & 44.8 & 68.0 & 48.6 \\
% \arrayrulecolor{white}\hline
\oursb & 110 & 856 
    & \textbf{51.3} & 70.4 & 55.7 & \textbf{44.6} & 68.0 & 48.2 
    & \textbf{52.0} & 70.5 & 56.4 & \textbf{45.2} & 68.2 & 49.3 \\
\arrayrulecolor{black}\hline

X101-64 & 140 & 972
    &- &- &- &- &- &-
    & 48.3 & 66.4 & 52.3 & 41.7 & 64.0 & 45.1 \\ % cswin
Swin-B & 145 & 982 
    & 50.8 & 70.1 & 55.1 & 43.9 & 67.4 & 47.4
    & 51.9 & 70.5 & 56.4 & 45.0 & 68.1 & 48.9 \\
ASMLP-B & 145 & 961 
    &- &- &- &- &- &-
    & 51.5 & 69.8 & 55.8 & 44.6 & 67.6 & 48.2 \\
\oursl & 134 & 902 
    & \textbf{51.8} & 70.9 & 56.3 & \textbf{44.8} & 68.4 & 48.4
    & \textbf{52.5} & 71.6 & 57.0 & \textbf{45.6} & 69.1 & 49.5 \\
\hline

\end{NiceTabular}
% }

\endgroup
