# Supplementary material for: Active Token Mixer
Source: arXiv:2203.06108 source file (2022-12-23)
Supplement: Supplementary file 4 [file supp_int_setting_back.tex]

\begingroup

% \resizebox{\textwidth}{!}{
\begin{NiceTabular}{c|c}
\hline
\Block{2-1}{Config} & Value \\
\cline{2-}
& xT, T, S, B, L \\
\hline

optimizer   & AdamW \\
learning rate & 1e-3 \\
weight decay & 0.05 \\ 
batch size  & 1024 \\
learning rate schedule & cosine decay \\
warmup epochs & 5 \\
training epochs & 300 \\
augmentation & \texttt{RandAug} (9, 0.5) \\
label smoothing \cite{szegedy2016InceptionV3} & 0.1 \\
mixup \cite{zhang2017mixup} & 0.8 \\
cutmix \cite{yun2019cutmix} & 1.0 \\
random erasing \cite{zhong2020randomerasing} & 0.25 \\
drop path \cite{huang2016deepdpr} & 0.1, 0.1, 0.2, 0.3, 0.3 \\
% exp. moving average (EMA) & 0.99996 \\
\hline

\end{NiceTabular}
% }

\vspace{-0.5cm}
\endgroup
