# Supplementary material for: Active Token Mixer
Source: arXiv:2203.06108 source file (2022-12-23)
Supplement: Supplementary file 5 [file supp_mask.tex]

\begingroup

\begin{NiceTabular}{@{}l|c@{\hspace{5pt}}c|ccc|ccc|ccc|ccc@{}}[code-before=
\rectanglecolor{\rc}{7-1}{7-15}
\rectanglecolor{\rc}{16-1}{16-15}
\rectanglecolor{\rc}{25-1}{25-15}
\rectanglecolor{\rc}{33-1}{33-15}
]
\hline
\multirow{2}{*}{Model}
& \multirow{2}{*}{\makecell{\#P.}} 
& \multirow{2}{*}{\makecell{FLOP}} 
& \multicolumn{6}{c}{Mask R-CNN 1$\times$} 
& \multicolumn{6}{c}{Mask R-CNN 3$\times$ MS} \\
% \cline{4-15}

& & & AP$^b$ & AP$^b_{50}$ & AP$^b_{75}$ & AP$^m$ & AP$^m_{50}$ & AP$^m_{75}$ & AP$^b$ & AP$^b_{50}$ & AP$^b_{75}$ & AP$^m$ & AP$^m_{50}$ & AP$^m_{75}$ \\
\hline

% & & & & & &
% & - & - & - & - & - & -

ResNet-18 & 31 & 207  % fp: our
    & 34.0 & 54.0 & 36.7 & 31.2 & 51.0 & 32.7
    & 36.9 & 57.1 & 40.0 & 33.6 & 53.9 & 35.7 \\ % pvt
PVT-T & 33 & 208 % fp: wave
    & 36.7 & 59.2 & 39.3 & 35.1 & 56.7 & 37.3 
    & 39.8 & 62.2 & 43.0 & 37.4 & 59.3 & 39.9 \\ % pvt
CycleMLP-B1  & 35 & 214 % flops: our
    & 39.4 & 61.4 & 43.0 & 36.8 & 58.6 & 39.1 
    & - & - & - & - & - & - \\ % wavemlp 
WaveMLP-T  & 35 & 215
    & 41.5 & 63.7 & 45.4 & 38.2 & 60.9 & 40.7
    & - & - & - & - & - & - \\ % wavemlp
\oursxt & 35 & 215
    & \textbf{42.8} & 64.9 & 46.9 & \textbf{39.5} & 62.1 & 42.5
    & \textbf{45.0} & 67.4 & 49.5 & \textbf{41.1} & 64.4 & 44.2 \\ 
\hline

ResNet-50 & 44 & 260 % wave 
    & 38.0 & 58.6 & 41.4 & 34.4 & 55.1 & 36.7
    & 41.0 & 61.7 & 44.9 & 37.1 & 58.4 & 40.1 \\  % cswin
PVT-S & 44 & 245 % cswin 
    & 40.4 & 62.9 & 43.8 & 37.8 & 60.1 & 40.3 
    & 43.0 & 65.3 & 46.9 & 39.9 & 62.5 & 42.8 \\ % cswin
Swin-T & 48 & 264 % cswin
    & 42.2 & 64.6 & 46.2 & 39.1 & 61.6 & 42.0 
    & 46.0 & 68.2 & 50.2 & 41.6 & 65.1 & 44.8 \\ % cswin
TwinsP-S & 44 & 245 % cswin 
    & 42.9 & 65.8 & 47.1 & 40.0 & 62.7 & 42.9 
    & 46.8 & 69.3 & 51.8 & 42.6 & 66.3 & 46.0 \\ % cswin
Twins-S & 44 & 228 % cswin
    & 43.4 & 66.0 & 47.3 & 40.3 & 63.2 & 43.4 
    & 46.8 & 69.2 & 51.2 & 42.6 & 66.3 & 45.8 \\ % cswin
% PVTv2-B2 \cite{wang2021pvtv2} & 45 & - 
    % & 45.3 & 67.1 & 49.6 & 41.2 & 64.2 & 44.4 
    % & & & & & & \\ % pvtv2
% ViL-S \cite{zhang2021ViL} & 45 % csin
%     & 44.9 & 67.1 & 49.3 & 41.0 & 64.2 & 44.1 
%     & 36 % github
%     & 44.2 & 65.2 & 47.6 & 28.8 & 48.0 & 57.8 \\ 
ASMLP-T & 48 & 260
    &- &- &- &- &- &-
    & 46.0 & 67.5 & 50.7 & 41.5 & 64.6 & 44.5 \\ % asmlp
CycleMLP-B2 & 47 & 250  % wave
    & 42.1 & 64.0 & 45.7 & 38.9 & 61.2 & 41.8 
    &- &- &- &- &- &- \\ % cycle
WaveMLP-S  & 47 & 250
    & 44.0 & 65.8 & 48.2 & 40.0 & 63.1 & 42.9 
    &- &- &- &- &- &- \\ % wavemlp
% Shift-T \cite{wang2022shift} & 48 & -
%     & 45.4 & -    & -    & 40.9 & -    & - 
%     & 47.1 & - & - & 42.3 & - & - \\ % shift
\ourst & 47 & 251
    & \textbf{44.8} & 66.9 & 49.0 & \textbf{41.0} & 64.2 & 44.3
    & \textbf{47.1} & 69.0 & 51.7 & \textbf{42.7} & 66.5 & 46.0 \\ % done
\hline

ResNet-101 & 63 & 336 % cswin
    & 40.4 & 61.1 & 44.2 & 36.4 & 57.7 & 38.8
    & 42.8 & 63.2 & 47.1 & 38.5 & 60.1 & 41.3 \\
PVT-M & 64 & 302  % cswin
    & 42.0 & 64.4 & 45.6 & 39.0 & 61.6 & 42.1
    & 44.2 & 66.0 & 48.2 & 40.5 & 63.1 & 43.5 \\
TwinsP-B & 64 & 302 % cswin
    & 44.6 & 66.7 & 48.9 & 40.9 & 63.8 & 44.2
    & 47.9 & 70.1 & 52.5 & 43.2 & 67.2 & 46.3 \\
% ViL-M \cite{zhang2021ViL} & 60  % csin
%     & 43.4 & - & - & 39.7 & - & - 
%     & -
%     & - &- &- &- &- &- \\
Swin-S  & 69 & 354 % cswin
    & 44.8 & 66.6 & 48.9 & 40.9 & 63.4 & 44.2
    & 48.5 & 70.2 & 53.5 & 43.3 & 67.3 & 46.6 \\
Twins-B & 76 & 340 % cswin
    & 45.2 & 67.6 & 49.3 & 41.5 & 64.5 & 44.8
    & 48.0 & 69.5 & 52.7 & 43.0 & 66.8 & 46.6 \\
ASMLP-S & 69 & 346
    & - & - & - & - & - & - 
    & 47.8 & 68.9 & 52.5 & 42.9 & 66.4 & 46.3 \\
CycleMLP-B3 & 58 & 310 % wave
    & 43.4 & 65.0 & 47.7 & 39.5 & 62.0 & 42.4
    &- &- &- &- &- &-  \\
WaveMLP-M & 60 & 312
    & 45.3 & 67.0 & 49.5 & 41.0 & 64.1 & 44.1
    &- &- &- &- &- &-  \\
% \ourss & 58 & 311
%     & 46.0 & 68.2 & 50.4 & 42.0 & 65.3 & 45.5
%     & 48.1 & 69.7 & 52.9 & 43.4 & 67.2 & 46.7 \\
% \arrayrulecolor{white}\hline
\oursb & 72 & 377
    & \textbf{46.5} & 68.6 & 51.0 & \textbf{42.5} & 66.1 & 45.8 
    & \textbf{48.7} & 70.4 & 53.5 & \textbf{43.8} & 67.7 & 47.4 \\
\arrayrulecolor{black}\hline

X101-64  & 102 & 493 
    & 42.8 & 63.8 & 47.3 & 38.4 & 60.6 & 41.3
    & 44.4 & 64.9 & 48.8 & 39.7 & 61.9 & 42.6  \\ % cswin
PVT-L  & 81 & 364 % cswin
    & 42.9 & 65.0 & 46.6 & 39.5 & 61.9 & 42.5 
    & 44.5 & 66.0 & 48.3 & 40.7 & 63.4 & 43.7  \\
% ViL-B \cite{zhang2021ViL} & 76 % csin
%     & 45.1 & - & - & 41.0 & - & - 
%     & 
%     & 45.7 & 67.2 & 49.9 & 41.3 & 64.4 & 44.5 \\
TwinsP-L & 81 & 364
    & 45.4 & - & - & 41.5 & - & -
    &-& -&- &- &- &- \\
Twins-L & 120 & 474
    & 45.9 & - & - & 41.6 & - & -
    & - &- &- &- &- &-  \\
Swin-B & 107 & 496
    & 45.5 & - & - & 41.3 & - & - % twins
    & 48.5 & 69.8 & 53.2 & 43.4 & 66.8 & 46.9  \\
% CycleMLP-B4 \cite{chen2022cyclemlp} & 72 % wave | flops: our
%     & 44.1 & 65.7 & 48.1 & 40.2 & 62.7 & 43.5
%     & 62
%     & 43.2 & 63.9 & 46.2 & 26.6 & 46.5 & 57.4 \\
CycleMLP-B5 & 95 & 421 % wave
    & 44.1 & 65.5 & 48.4 & 40.1 & 62.8 & 43.0
    &- &- &- &- &- &-   \\
WaveMLP-B & 75 & 353
    & 45.7  & 67.5 & 50.1 & 27.8 & 49.2 & 59.7
    &- &- &- &- &- &-  \\

\oursl & 96 & 424
    & \textbf{47.4} & 69.9 & 52.0 & \textbf{43.2} & 67.3 & 46.5
    & \textbf{48.7} & 70.5 & 53.3 & \textbf{43.7} & 67.4 & 47.2 \\

\hline

\end{NiceTabular}

\endgroup
