# Supplementary material for: Active Token Mixer
Source: arXiv:2203.06108 source file (2022-12-23)
Supplement: Supplementary file 6 [file supp_retina.tex]

\begingroup

\begin{NiceTabular}{@{}l|c@{\hspace{5pt}}c|ccc|ccc|ccc|ccc@{}}[code-before=
\rectanglecolor{\rc}{7-1}{7-15}
\rectanglecolor{\rc}{15-1}{15-15}
\rectanglecolor{\rc}{23-1}{23-15}
\rectanglecolor{\rc}{31-1}{31-15}
]
\hline
\multirow{2}{*}{Model}
& \multirow{2}{*}{\makecell{\#P.}} 
& \multirow{2}{*}{\makecell{FLOPs}} 
& \multicolumn{6}{c}{RetinaNet 1$\times$} 
& \multicolumn{6}{c}{RetinaNet 3$\times$ MS} \\
& & 
& AP$^b$ & AP$^b_{50}$ & AP$^b_{75}$ 
& AP$_S$ & AP$_{M}$ & AP$_{L}$
& AP$^b$ & AP$^b_{50}$ & AP$^b_{75}$ 
& AP$_S$ & AP$_{M}$ & AP$_{L}$ \\
\hline

ResNet18  & 21 & 189
    & 31.8 & 49.6 & 33.6 & 16.3 & 34.3 & 43.2
    & 35.4 & 53.9 & 37.6 & 19.5 & 38.2 & 46.8 \\ % pvt
PVT-T  & 23 & 190
    & 36.7 & 56.9 & 38.9 & 22.6 & 38.8 & 50.0
    & 39.4 & 59.8 & 42.0 & 25.5 & 42.0 & 52.1 \\ % pvt
% ViL-T \cite{zhang2021ViL} & 27  % csin
%     & 41.4 & 63.5 & 45.0 & 24.5 & 44.5 & 55.4 
%     & 17
%     & 40.7 & 61.3 & 43.3 & 26.7 & 44.8 & 53.6 \\
CycleMLP-B1  & 25 & 195
    & 38.6 & 59.1 & 40.8 & 21.9 & 41.8 & 50.7  
    & - & - & - & - & - & - \\ % wavemlp 
WaveMLP-T  & 25 & 196
    & 40.4 & 61.0 & 43.4 & 24.9 & 43.7 & 51.7
    & - & - & - & - & - & - \\ % wavemlp
\oursxt & 25 & 196
    & \textbf{41.2} & 62.3 & 43.7 & 24.4 & 45.3 & 54.2 
    & \textbf{43.7} & 64.7 & 46.7 & 28.9 & 47.4 & 57.4 \\ % done
\hline

ResNet-50  & 38 & 239
    & 36.3 & 55.3 & 38.6 & 19.3 & 40.0 & 48.8 
    & 39.0 & 58.4 & 41.8 & 22.4 & 42.8 & 51.6 \\% twins
PVT-S  & 34 & 227 
    & 40.4 & 61.3 & 43.0 & 25.0 & 42.9 & 55.7 
    & 42.2 & 62.7 & 45.0 & 26.2 & 45.2 & 57.2 \\% ppvt
Swin-T  & 39 & 245 
    & 41.5 & 62,1 & 44.2 & 25.1 & 44.9 & 55.5
    & 45.0 & 65.9 & 48.4 & 29.7 & 48.9 & 58.1\\ % focal
TwinsP-S  & 34 & 286
    & 43.0 & 64.1 & 46.0 & 27.5 & 46.3 & 57.3 
    & 45.2 & 66.5 & 48.6 & 30.0 & 48.8 & 58.9 \\% twins
Twins-S  & 34 & 236
    & 43.0 & 64.2 & 46.3 & 28.0 & 46.4 & 57.5 
    & 45.6 & 67.1 & 48.6 & 29.8 & 49.3 & 60.0 \\%twins
% PVTv2-B2 \cite{wang2021pvtv2} & 45 & - 
    % & 45.3 & 67.1 & 49.6 & 41.2 & 64.2 & 44.4 
    % & & & & & & \\ % pvtv2
CycleMLP-B2  & 37 & 231
    & 40.9 & 61.8 & 43.4 & 23.4 & 44.7 & 53.4
    & - & - & - & - & - & - \\ % cycle
WaveMLP-S   & 37 & 231
    & 43.4 & 64.4 & 46.5 & 26.6 & 47.1 & 57.1
    & - & - & - & - & - & -  \\ % wavemlp
\ourst & 37 & 233
    & \textbf{43.6} & 64.9 & 46.8 & 27.2 & 47.5 & 57.9
    & \textbf{45.8} & 66.9 & 49.2 & 29.9 & 49.3 & 59.9 \\ % done
\hline

ResNet-101  & 57 & 315
    & 38.5 & 57.8 & 41.2 & 21.4 & 42.6 & 51.1
    & 40.9 & 60.1 & 44.0 & 23.7 & 45.0 & 53.8 \\
PVT-M  & 54 & 283
    & 41.9 & 63.1 & 44.3 & 25.0 & 44.9 & 57.6 
    & 43.2 & 63.8 & 46.1 & 27.3 & 46.3 & 58.9 \\
TwinsP-B  & 54 & 374
    & 44.3 & 65.6 & 47.3 & 27.9 & 47.9 & 59.6
    & 46.4 & 67.7 & 49.8 & 31.3 & 50.2 & 61.4 \\
% ViL-M \cite{zhang2021ViL} & 60  % csin
%     & 43.4 & - & - & 39.7 & - & - 
%     & -
%     & - &- &- &- &- &- \\
Swin-S  & 60 & 335
    & 44.5 & 65.7 & 47.5 & 27.4 & 48.0 & 59.9 
    & 46.4 & 67.0 & 50.1 & 31.0 & 50.1 & 60.3\\%focal
Twins-B & 67 & 376
    & 45.3 & 66.7 & 48.1 & 28.5 & 48.9 & 60.6
    & \textbf{46.9} & 68.0 & 50.2 & 31.7 & 50.3 & 61.8 \\
CycleMLP-B3  & 48 & 291
    & 42.5 & 63.2 & 45.3 & 25.2 & 45.5 & 56.2 
    & - &- &- &- &- &- \\
WaveMLP-M  & 49 & 291
    & 44.8 & 65.8 & 47.8 & 28.0 & 48.2 & 59.1 
    & - &- &- &- &- &- \\
% \ourss & 48 & 293
%     & \textbf{45.4} & 66.7 & 48.5 & 28.3 & 49.7 & 59.7 
%     & {46.3} & 68.0 & 49.5 & 30.4 & 50.6 & 59.9 \\
% \arrayrulecolor{white}\hline
\oursb & 62 & 359
    & \textbf{45.6} & 67.2 & 48.9 & 28.9 & 49.6 & 60.5 
    & {46.6} & 67.7 & 50.1 & 30.4 & 50.4 & 61.0 \\
\arrayrulecolor{black}\hline

X101-64  & 96 &473
    & 41.0 & 60.9 & 44.0 & 23.9 & 45.2 & 54.0
    & 41.8 & 61.5 & 44.4 & 25.2 & 45.4 & 54.6\\%focal
PVT-L  & 71 & 345
    & 42.6 & 63.7 & 45.4 & 25.8 & 46.0 & 58.4
    & 43.4 & 63.6 & 46.1 & 26.1 & 46.0 & 59.5 \\
% ViL-B \cite{zhang2021ViL} & 76 % csin
%     & 45.1 & - & - & 41.0 & - & - 
%     & 
%     & 45.7 & 67.2 & 49.9 & 41.3 & 64.4 & 44.5 \\
TwinsP-L  & 71 & 476
    & 45.1 & 66.4 & 48.4 & - & - & - 
    & - &- &- &- &- &- \\
Twins-L  & 111 & 528
    & 45.7 & 67.1 & 49.2 & - & - & - 
    & - &- &- &- &- &- \\
Swin-B  & 98 & 477
    & 44.7 & 65.9 & 47.8 & - & - & - 
    & 45.8 & 66.4 & 49.1 & 29.9 & 49.4 & 60.3 \\
% CycleMLP-B4  & 72 % wave | flops: our
%     & 44.1 & 65.7 & 48.1 & 40.2 & 62.7 & 43.5
%     & 62
%     & 43.2 & 63.9 & 46.2 & 26.6 & 46.5 & 57.4 \\
CycleMLP-B5  & 86 & 402
    & 42.7 & 63.3 & 45.3 & 24.1 & 46.3 & 57.4  
    & - &- &- &- &- &- \\
WaveMLP-B  & 66 & 334
    & 44.2 & 65.1 & 47.1 & 27.1 & 47.8 & 58.9 
    & - &- &- &- &- &- \\
\oursl & 86 & 405
    & \textbf{46.1} & 67.4 & 49.4 & 29.9 & 50.1 & 61.0 
    & \textbf{47.5} & 68.8 & 51.2 & 31.5 & 51.4 & 62.0 \\
\hline

\end{NiceTabular}
\endgroup
